# Supplementary material for: Recurrent Attention-based Token Selection for Efficient Streaming Video-LLMs
Source: arXiv:2510.17364 source file (2025-10-20)
Supplement: Supplementary file 2 [file position.tex]

\begin{table}[h]
\caption{Accuracy on NextQA validation set for different percentage (\%) of visual tokens selected with the proposed attention-based method.}
\centering
\begin{tabular}{cc}
\toprule
\textbf{Selected Visual Tokens} & \textbf{Acc. on NextQA-valset (\%)} \\
\midrule
$1\%$ & 68.0 \\
$6\%$ & 77.0\\
$12\%$ &  78.4\\
$19\%$ &  78.7\\
$25\%$ &  79.0 \\
$100\%$ & 78.6 \\
\bottomrule
\end{tabular}
\label{tab:position}
\end{table}
